# Supplementary material for: GILE: A Generalized Input-Label Embedding for Text Classification
Source: arXiv:1806.06219 source file (2019-01-30)
Supplement: Supplementary file 1 [file appendix.tex]

\section{APPENDIX}

\begin{table*}
  \small
  \centering
  {\tabcolsep=3.2pt
  \begin{tabular}{ p{0.4cm}  p{0.2cm} l | c c c c c c c | c c c c c c c | c}
	\hline
	&    \multicolumn{2}{c|}{{   \textbf{Models}}}  & \multicolumn{7}{c|}{{   \textbf{Languages (en + aux $\rightarrow$ en)}}}  & \multicolumn{7}{c|}{{   \textbf{Languages (en + aux $ \rightarrow$ aux)} }} & \multicolumn{1}{c}{{   \textbf{Stat.} }} \\
  \rowcolor{white}   &  \multicolumn{2}{c|}{{ abbrev. }} & de  & es  & pt & uk & ru & ar & fa & de & es & pt & uk & ru & ar & fa & \textit{avg} \\ \hline\hline
  \parbox[t]{1mm}{\multirow{6}{*}{\rotatebox[origin=c]{90}{ Baselines }}} &  \parbox[t]{2mm}{\multirow{3}{*}{\rotatebox[origin=c]{90}{  Mono  }}}  &  NN (Avg)  & \multicolumn{7}{c|}{ \rule[0.25em]{0.3\columnwidth}{0.3pt} 24.4 \rule[0.25em]{0.3\columnwidth}{0.3pt} }  & 21.8 & 22.1 & 24.3 & 33.0 & 26.0 & 24.1 & 32.1 & 25.3 \\
   & & HNN (Avg) &  \multicolumn{7}{c|}{ \rule[0.25em]{0.3\columnwidth}{0.3pt} 39.3 \rule[0.25em]{0.3\columnwidth}{0.3pt} } & 39.6 & 37.9 & 33.6 & 42.2 & 39.3 & 34.6 & 43.1 & 38.9\\
    &  & HAN (Att)  &  \multicolumn{7}{c|}{ \rule[0.25em]{0.3\columnwidth}{0.3pt} 43.4 \rule[0.25em]{0.3\columnwidth}{0.3pt} } & 44.8 & 46.3 & 41.9 & 46.4 & 45.8 & 41.2 & {49.4} & 44.2 \\ \cline{2-18}
  &  \parbox[t]{2mm}{\multirow{3}{*}{\rotatebox[origin=c]{90}{  Multi  }}}  & MHAN-Enc  & 45.4 & 45.9 & {44.3} & 41.1 & 42.1 & {44.9} & 41.0 & 43.9 & 46.2 & 39.3 & 47.4 & 45.0 & 37.9 & 48.6  & 43.8\\
& & MHAN-Att &  {46.3} & {46.0} & {45.9} & {45.6} & {46.4} & {46.4} & {46.1} & {46.5} & {46.7} & {43.3} & {47.9} & {45.8} & {41.3} & 48.0 & \textcolor{blue}{45.8} \\
& &  MHAN-Both &  45.7 & 45.6 & 41.5 & 41.2 & 45.6 & {44.6} & {43.0} & 45.9 & 46.4 & 40.3 & 46.3 & {46.1} & 40.7 & {50.3} & 44.5\\
\hline
\parbox[t]{1mm}{\multirow{6}{*}{\rotatebox[origin=c]{90}{  Ours }}} &  \parbox[t]{2mm}{\multirow{3}{*}{\rotatebox[origin=c]{90}{  Mono  }}}  & LA-NN (Avg)  & \multicolumn{7}{c|}{ \rule[0.25em]{0.3\columnwidth}{0.3pt} \textbf{27.5} \rule[0.25em]{0.3\columnwidth}{0.3pt} }  & \textbf{27.5} & \textbf{28.4}  & \textbf{29.2}  & \textbf{36.8}  & \textbf{31.6}  & \textbf{32.1}  & \textbf{35.6} &  \textbf{29.5}\\
 & & LA-HNN (Avg) &  \multicolumn{7}{c|}{ \rule[0.25em]{0.3\columnwidth}{0.3pt}  \textbf{43.1} \rule[0.25em]{0.3\columnwidth}{0.3pt} } &  \textbf{43.4} & \textbf{42.0}  &  \textbf{37.7}  &   \textbf{43.0}  & \textbf{42.9} &  \textbf{36.6}  &  \textbf{44.1} & \textbf{42.2}\\
  &  & LA-HAN (Att)  &  \multicolumn{7}{c|}{ \rule[0.25em]{0.3\columnwidth}{0.3pt}  \textbf{45.9}  \rule[0.25em]{0.3\columnwidth}{0.3pt} }  & \textbf{47.3} &  \textbf{47.4} & \textbf{42.6} &  \textbf{46.6}   & \textbf{46.9}  & \textbf{41.9}  & 48.6 & \textbf{45.9}\\ \cline{2-18}
&  \parbox[t]{2mm}{\multirow{3}{*}{\rotatebox[origin=c]{90}{  Multi  }}}  & LA-MHAN-Enc  & \textbf{46.0} &  \textbf{46.6} & 41.2  & \textbf{42.5} & {\textbf{46.4}}  & 43.4 & \textbf{41.8} & \textbf{47.2} &  \textbf{47.7} & \textbf{41.5}  & {\textbf{49.5}} & {\textbf{46.6}} &  \textbf{41.4} & {\textbf{50.7}} & \textbf{45.1}\\
& & LA-MHAN-Att & {\textbf{47.3}} & {\textbf{47.0}} & {\textbf{45.8}} & {\textbf{45.5}} & \textbf{46.2} & {\textbf{46.5}} & 45.5 & {\textbf{47.6}} & {\textbf{47.9}} & {\textbf{43.5}}& \textbf{49.1} & \textbf{46.5} &{\textbf{42.2}}  & \textbf{50.3} & \textcolor{blue}{\textbf{46.5}}\\
& &  LA-MHAN-Both& \textbf{47.0} &  {\textbf{46.7}} & {\textbf{42.8}} & {\textbf{42.0}} & \textbf{45.6}  & 42.8  & 39.3 & {\textbf{48.0}} & \textbf{47.6} &\textbf{43.1}  & \textbf{48.5} & 46.0 & \textbf{42.1} & 49.0 & \textbf{45.0} \\
\hline
\end{tabular}}
\caption{\label{full-rec_results-spe}Full-resource classification performance ($F_{1}$) on specific topic categories using monolingual and bilingual models with \textsc{dense} encoders on English as target (left) and the auxiliary language as target (right).  The average bilingual F1-score is noted  \textit{avg} and the top average scores are marked in \textcolor{blue}{blue}.
}
\end{table*}

\subsection{Additional Results}
Table \ref{full-rec_results-spe} displays the results of full-resource document classification using \textsc{DENSE} encoders for specific labels.  On the left, the performance of models on the English sub-corpus  is  shown  when  English  and  an auxiliary sub-corpus are used for training, and on the right,  the  performance  on  the  auxiliary sub-corpus is shown when that sub-corpus and the English sub-corpus are used for training. The main observations and conclusions are the same as what was presented in Section \ref{dwres}.
